# Supplementary material for: Omni-Life: Benchmarking Omnimodal Real-Time AI Assistants in People's Daily Lives
Source: arXiv:2611.02835 source file (2026-11-02)
Supplement: Supplementary file 1 [file contents.tex]

% The template suppresses contents entries. Enable only appendix headings.
\makeatletter
% Link to the recorded page top so deferred floats cannot separate a heading from its target.
\newcommand{\omni@appendixentry}[2]{%
    \addtocontents{toc}{\protect\contentsline{#1}{#2}{\thepage}{page.\thepage}\protected@file@percent}%
}
\renewcommand{\addcontentsline}[3]{%
    \def\omni@entrytype{#2}%
    \def\omni@sectiontype{section}%
    \def\omni@subsectiontype{subsection}%
    \ifx\omni@entrytype\omni@sectiontype
        \omni@appendixentry{#2}{#3}%
    \else
        \ifx\omni@entrytype\omni@subsectiontype
            \omni@appendixentry{#2}{#3}%
        \fi
    \fi
}

% Keep this compact navigation block together as it flows with the text.
\par\noindent
\begin{minipage}{\linewidth}
\section*{Appendix Contents}
\begingroup
    \hypersetup{linktoc=all}
    \setcounter{tocdepth}{2}
    \setlength{\parskip}{0pt}
    \setlength{\cftbeforesecskip}{0.55\baselineskip}
    \setlength{\cftbeforesubsecskip}{0.1\baselineskip}
    \setlength{\cftsecnumwidth}{1.5em}
    \setlength{\cftsubsecindent}{1.5em}
    \setlength{\cftsubsecnumwidth}{2.4em}
    \@starttoc{toc}
\endgroup
\end{minipage}
\par
\makeatother
